# Supplementary material for: Verified Rust Monitors for Lola Specifications
Source: arXiv:2012.08961 source file (2020-12-15)
Supplement: Supplementary file 1 [file appendix.tex]

%\section{Code Generation}
%
%\Cref{fig:monitorstructure_full} shows the complete template for the monitor implementation.
%
%\begin{figure}[t]
%  \input{figures/codestructure}
%  \caption{TODO Change Colors as well!}
%  \label{fig:monitorstructure_full}
%\end{figure}

\section{Specifications}\label{app:specs}

The specifications used for the experimental evaluation can be found here.

\Cref{fig:networkspec} contains the network specification~\cite{fpgalola}.
The specification monitors the network traffic of a server based on the source and destination IP of requests, TCP flags, and the length of the payload.
It counts the number of incoming connections and computes the workload, \ie, the number of bytes received over push requests.
If any of these numbers exceeds a threshold, it raises and alarm.
Moreover, it keeps track of the number of open connections.  
A trigger indicates when the the server attempts to close a connection even though none is open.

% Flight Phase Detection Spec

The second specification~\cite{uav2} (\Cref{fig:flightphasespec}) detects different flight phases of a drone and raises an alarm if actual velocity and reference velocity deviate. 
First, the minimal and maximal velocities are computed. 
If their deviation exceeds a given threshold, these computations are reset. 
The specification counts how many steps no reset has taken place. 
Intuitively, this is used to detect whether the drone is accelerating or hovering / keeping its velocity steady.
Second, deviations between the actual velocity and the reference velocity, given by the flight controller, are detected. 
The specification monitors the worst deviation and raises an alarm if it exceeds a given threshold. 
Note that the computation of the velocity requires a square root.
Since this operation is not supported, we left it out for the verification. 
Alternatively, the compiler could introduce a \lstinline{sqrt} function and mark it as \emph{trusted}, this would indicate \viper that the function is correct as is and thus does not need to be verified.

% Network Spec
\begin{lstlisting}[
  style=LolaDefault,
  float,
  floatplacement=t,
  caption=\lola specification for monitoring network traffic,
  label=fig:networkspec
]
input src: Int32, dst: Int32
input fin: Bool, push: Bool, syn: Bool
input length: Int32
constant server: Int32 := 213451

output count : Int32 := ite(count[-1,0] > 201, 0, count[-1,0] + 1)
output receiver : Int32 := ite(dst==server, receiver[-2,0] + 2, ite(count > 200, 0, receiver[-1,0]))
trigger receiver > 50 "Many incoming connections."

output received : Int32 := ite(dst==server && push, 0, length)
output workload : Int32 := ite(count > 200, workload[-1,0] + 1, 0)
trigger workload > 25 "Workload too high."

output opened : Int32 := opened[-1,0] + ite(dst==server && syn, 1, 0)
output closed : Int32 := closed[-1,0] + ite(dst==server && fin, 1, 0)
trigger opened - closed < 0 "Closed more connections than have been opened."
\end{lstlisting}

\begin{lstlisting}[
style=LolaDefault,
caption=\lola specification for flight phase detection,
label=fig:flightphasespec,
float,
floatplacement=t,
]
input vel_x: Int32, vel_y: Int32, vel_r_x: Int32, vel_r_y: Int32

output velocity : Int32 := vel_x*vel_x + vel_y*vel_y
output velocity_max : Int32 := ite(reset_max[-1,false], velocity, ite(velocity_max[-1,0] > velocity, velocity_max[-1,0], velocity))
output velocity_min : Int32 := ite(reset_max[-1,false], velocity, ite(velocity_min[-1,0] < velocity, velocity_min[-1,0], velocity))
output dif_max : Int32 := velocity_max - velocity_min
output reset_max: Bool := dif_max > 1
output unchanged: Int32 := ite(reset_max[-1,false], 0, unchanged[-1,0] + 1)
output vel_dev : Int32 := vel_r_x - vel_x + vel_r_y - vel_y
output worst_dev: Int32 := ite(unchanged > 15, vel_dev, ite(worst_dev[-1,-10] < vel_dev, vel_dev, worst_dev[-1,-10]))

trigger vel_dev > 10 "Deviation between actual und reference velocity too high."
trigger worst_dev > 20 "Worst deviation between actual und reference velocity too high."
\end{lstlisting}
